# Supplementary material for: Leveraging Passage Retrieval with Generative Models for Open Domain Question Answering
Source: arXiv:2007.01282 source file (2021-02-03)
Supplement: Supplementary file 1 [file appendix.tex]

\appendix
\begin{table*}[t]
\centering
\begin{tabular}{lcccc}
  \toprule
  Model & NaturalQuestions & \multicolumn{2}{c}{TriviaQA} & SQuAD Open \\
  \midrule
  DrQA~\citep{chen2017reading}             & -    & -    & -    & 29.8 \\
  Multi-Passage BERT~\citep{wang2019multi} & -    & -    & -    & 53.0 \\ 
  Path Retriever~\citep{asai2019learning}  & 31.7 & -    & -    & \textbf{56.5} \\
  Graph Retriever~\citep{min2019knowledge} & 34.7 & 55.8 & -    & - \\
  Hard EM~\citep{min2019discrete}          & 28.8 & 50.9 & -    & - \\
  ORQA~\citep{lee2019latent}               & 31.3 & 45.1 & -    & 20.2 \\
  REALM~\citep{guu2020realm}               & 40.4 & -    & -    &  \\
  DPR~\citep{karpukhin2020dense}           & 41.5 & 57.9 & -    & 36.7 \\
  SpanSeqGen~\citep{min2020ambigqa}        & 42.5 & -    & -    & - \\
  RAG~\citep{lewis2020retrieval}           & 44.5 & 56.1 & 68.0 & - \\
  \midrule
  T5~\citep{roberts2020much} & 36.6 & - & 60.5 & - \\
  GPT-3 few shot~\citep{brown2020language}    & 29.9 & - & 71.2 & - \\
  \midrule
  Fusion-in-Decoder (base)    & 48.2 & 65.0 & 77.1 & 53.4 \\
  Fusion-in-Decoder (large)   & \textbf{51.4} & \textbf{67.6} & \textbf{80.1} & \textbf{56.7} \\
  \bottomrule
\end{tabular}
\caption[Caption]{Comparison to state-of-the-art. On TriviaQA, we report results on the open domain test set (left), and on the hidden test set (right). }%, \url{competitions.codalab.org/competitions/17208\#results}).}
\label{tab:appendix_results}
\end{table*}

\section{Experimental Details}
\paragraph{Datasets.}
We follow the standard open domain question answering setup from~\cite{lee2019latent}, and briefly describe it here.
We use the validation as test, and keep 10\% of the training set for validation. The format of the three datasets used are slightly different, in the following we detail the specificities of each dataset. 

For NaturalQuestions, as well as SQuAD, each question is associated with a list of acceptable answers. During training, we sample the training target from this list at each gradient step. The open-domain version of NaturalQuestions is obtained from the original version of the dataset by discarding answers with more than 5 tokens.

For TriviaQA, the \emph{unfiltered} version is used for open-domain question answering. For this dataset there is both a human generated answer and a list of acceptable answers. We use the human generated answer as a training target. Answers in uppercase are normalized by converting all letters in lowercase except the first letter of each word, using the \texttt{title} Python string method.
\paragraph{Training.} The Fusion-in-Decoder model is initialized with a pretrainined T5 model. We fine-tune the models on each dataset independently, using the Adam algorithm with a constant learning rate of $10^{-4}$ and a dropout rate of 10\%.
We train the model for 10k gradient steps, with a batch size of 64.
We evaluate models every 500 steps and select the best one on the validation set based on the Exact Match score.

\section{Results}
See Table~\ref{tab:appendix_results} for more exhaustive comparison of the performance of the different methods mentioned in our paper.
